# Supplementary material for: Blind Motion Deblurring with Pixel-Wise Kernel Estimation via Kernel Prediction Networks
Source: arXiv:2308.02947 source file (2023-08-05)
Supplement: Supplementary file 2 [file supp_mat_kernels_masks.tex]

\section{Learning of Kernel Prediction Network}

Given a blurry image, the \textit{Kernel Prediction Network} predicts a basis of kernels and the corresponding mixing coefficients. The number of (kernels, mixing coefficients) pairs that can generate the estimated kernel is infinite. Since we are not interested in any particular pair, we just let the network learn how to predict the pair without any constraint. 

Previous motion estimation methods \cite{gong2017motion, zhang2021exposure} learn how to predict motion vectors by minimizing a re-blur loss. Since the estimation is local, and in many regions of the image there is not enough information to uniquely infer the motion vector, the motion map must be regularized. In contrast to those articles, we did not have to constrain the kernel basis nor the mixing coefficients to obtain smooths kernel maps. The reason that explains this behavior is that during training, we used a \textit{kernel loss} in addition to the \textit{reblur loss}.  

In \cref{fig:kernels_grid_different_losses}, we show the kernels estimated for crops in the GoPro dataset. The first columns show the kernels estimated when there is no \textit{kernel loss} during training. The kernels obtained are dotted. This may be by the combination of two factors: a) during training, there is not enough information to learn clearly delimited kernels b) the kernels in the GoPro dataset are \textit{dotted} due to blurry images generated by averaging consecutive frames. Adding the \textit{kernel loss} acts as a prior that contributes to generating continuous, well-shaped kernels. \cite{zhang2021exposure} compare different estimation methods using the reblur performance on the GoPro dataset. In \cref{tab:reblur_performance_NoFC}, we show the reblur performance for the methods trained with: a) \textit{reblur loss} on the GoPro dataset, b) kernels and reblur loss on the GoPro dataset and a synthetic dataset c) kernels and reblur loss only using the synthetic dataset. The reblur performance is much better when using the reblur loss on the GoPro dataset. However, the quality of the kernels improves considerably when adding the \textit{kernels loss}.  In \cref{fig:kernels_grid_Kohler} and  \cref{fig:kernels_grid_Lai}, we show the kernels map obtained on real images from the K\"{o}hler and the Lai dataset. Again, the kernels' better quality when using the \textit{kernels loss} is observed. 

\begin{figure}
    \centering
    \begin{tabular}{*{3}{c}} 
    (a) & (b) & (c) \\
    \includegraphics[trim= 0 0 0 0, clip,width=0.33\textwidth]{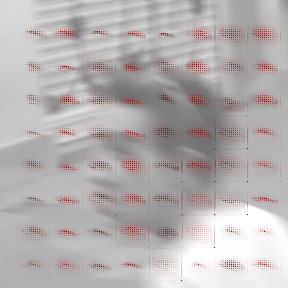} &
    \includegraphics[trim= 0 0 0 0, clip,width=0.33\textwidth]{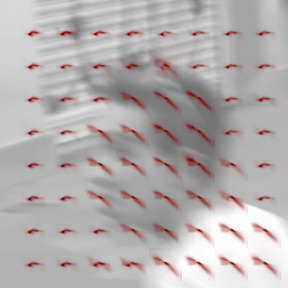}  &   
 \includegraphics[trim= 0 0 0 0, clip,width=0.33\textwidth]{imgs/kernels_masks/first_round/0249_kernels_grid.jpg}   \\
 \includegraphics[trim= 0 0 0 0, clip,width=0.33\textwidth]{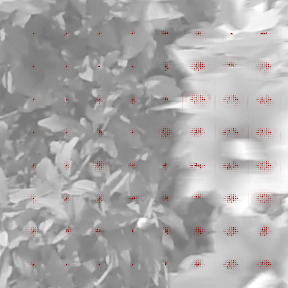} &
    \includegraphics[trim= 0 0 0 0, clip,width=0.33\textwidth]{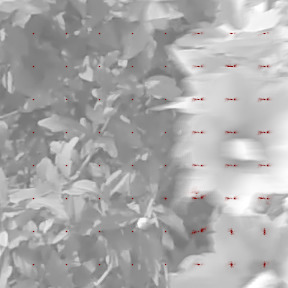}  &   
 \includegraphics[trim= 0 0 0 0, clip,width=0.33\textwidth]{imgs/kernels_masks/first_round/0316_kernels_grid.jpg}   
    \end{tabular}
    \caption{Caption}
    \label{fig:kernels_grid_different_losses}
\end{figure}

\begin{table}[]
    \centering
    \begin{tabular}{c|c|c}
         Training Set &  Loss  &  PSNR \\
         COCO         & Reblur + Kernels & 33.63 \\
         \hline
         GoPro &   Reblur & 38.64   \\
         GoPro + ADE &   Reblur + Kernels &  34.94  \\
         ADE &   Reblur  &    \\
         ADE &   Reblur + Kernels &    \\
    \end{tabular}
    \caption{Reblur performance with NoFC architecture}
    \label{tab:reblur_performance_NoFC}
\end{table}

\begin{table}[]
    \centering
    \begin{tabular}{c|c|c}
         Training Set &  Loss  &  PSNR \\
         GoPro &   Reblur &    \\
         GoPro + ADE &   Reblur + Kernels &  37.0  \\
         ADE &   Reblur  & 37.57   \\
         ADE &   Kernels  &  32.81  \\
         ADE &   Reblur + Kernels &    \\
    \end{tabular}
    \caption{Reblur performance with Xia architecture}
    \label{tab:reblur_performance_Xia}
\end{table}

\begin{figure}
    \centering
    \begin{tabular}{*{3}{c}} 
    (a) & (b) & (c) \\
    \includegraphics[trim= 0 0 0 0, clip,width=0.33\textwidth]{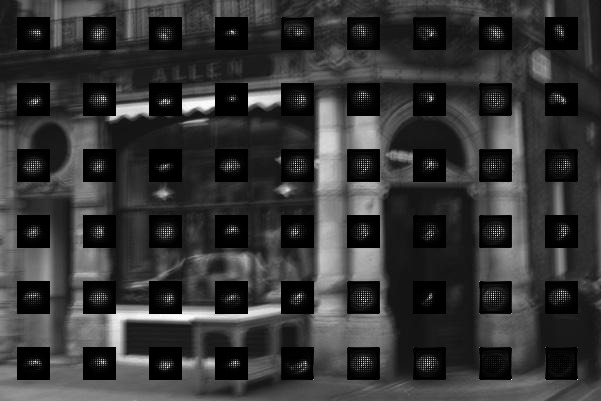} &
    \includegraphics[trim= 0 0 0 0, clip,width=0.33\textwidth]{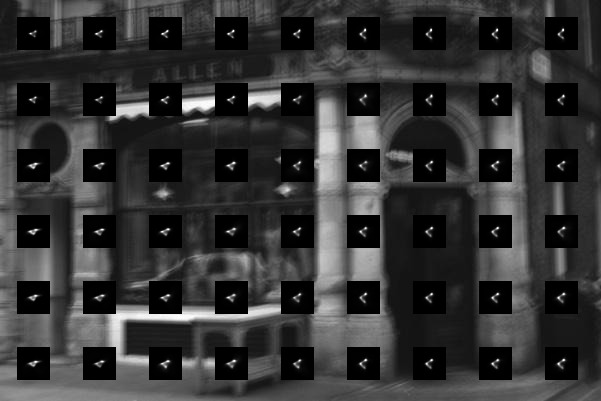}  &  
 \includegraphics[trim= 0 0 0 0, clip,width=0.33\textwidth]{imgs/kernels_masks/first_round/butchershop.jpg}   \\
 \includegraphics[trim= 0 0 0 0, clip,width=0.33\textwidth]{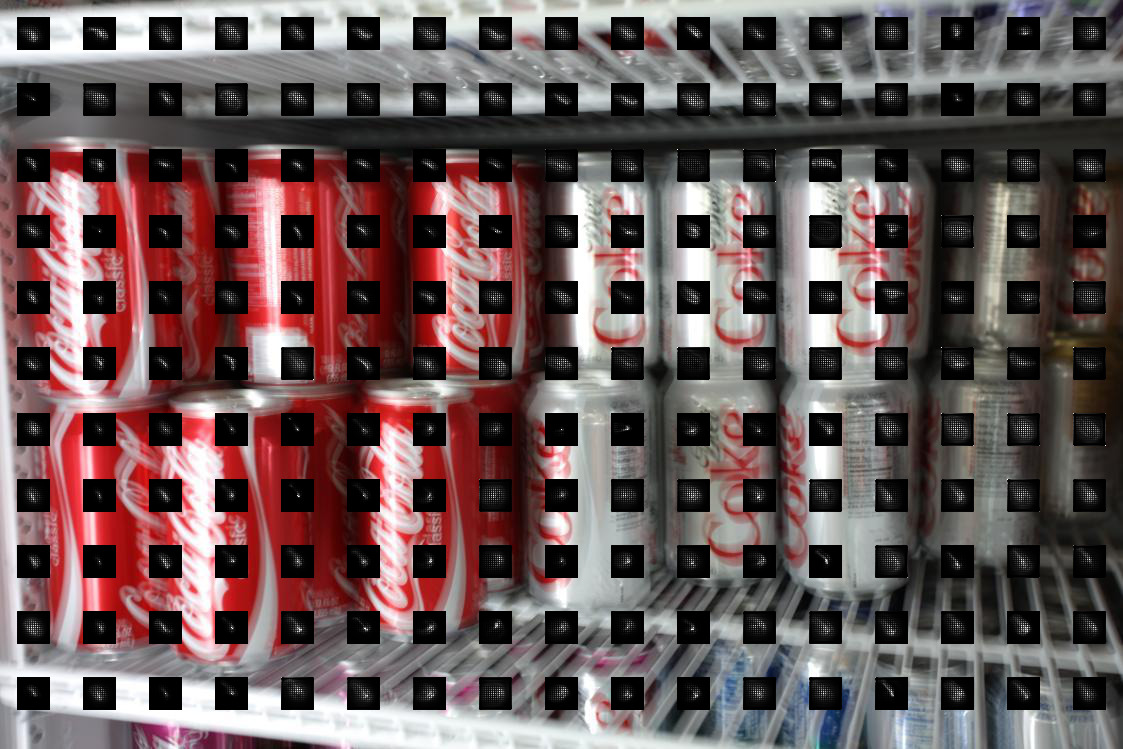} &
    \includegraphics[trim= 0 0 0 0, clip,width=0.33\textwidth]{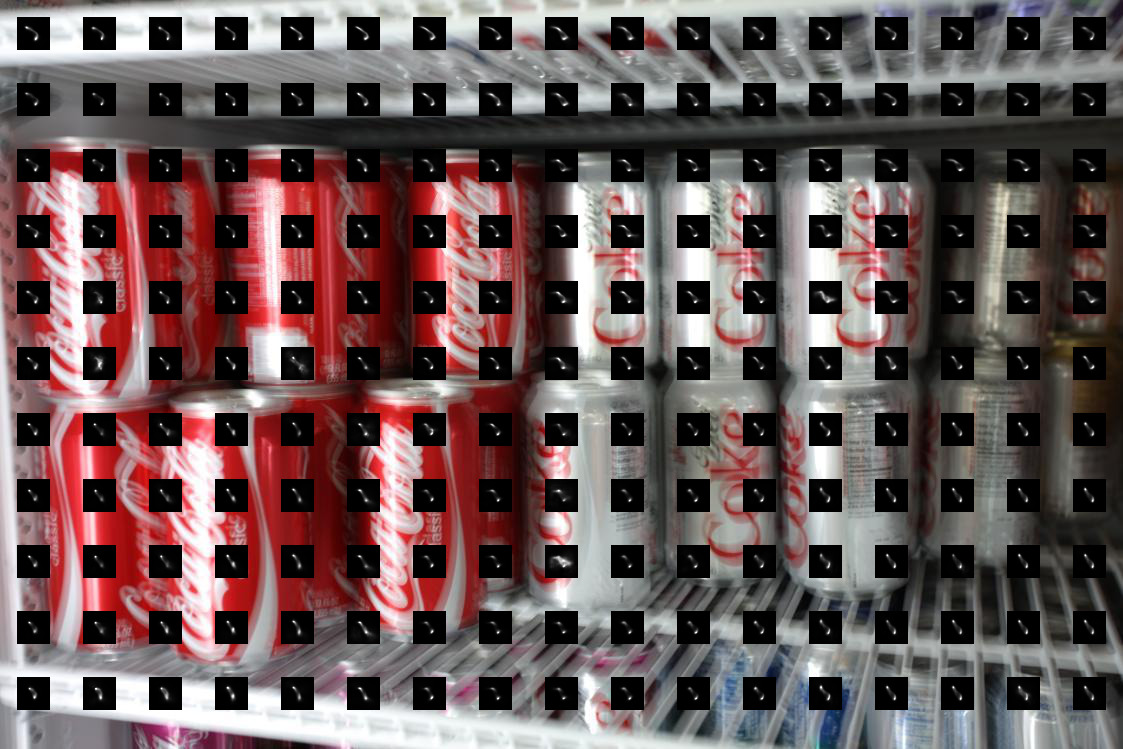}  &   
 \includegraphics[trim= 0 0 0 0, clip,width=0.33\textwidth]{imgs/kernels_masks/first_round/coke.jpg} \\
  \includegraphics[trim= 0 0 0 0, clip,width=0.33\textwidth]{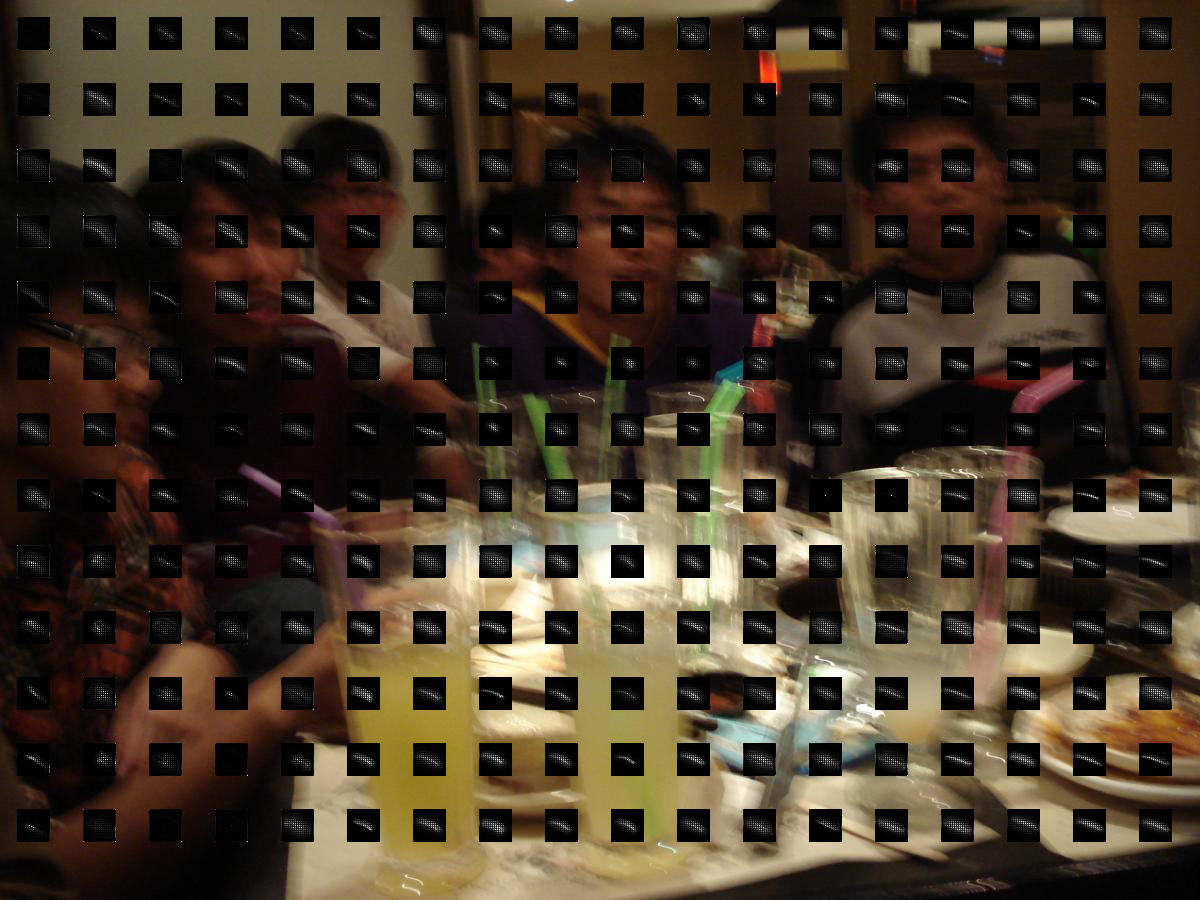} &
    \includegraphics[trim= 0 0 0 0, clip,width=0.33\textwidth]{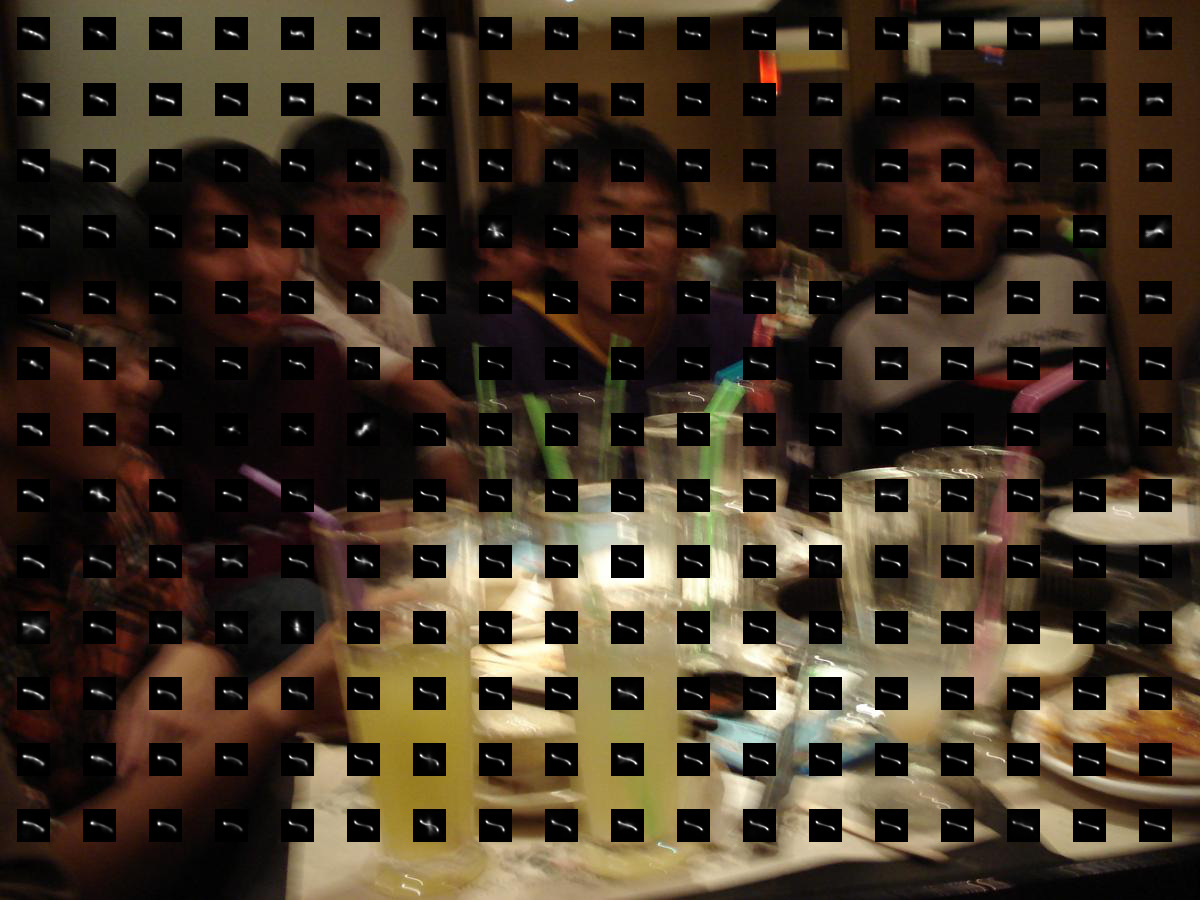}  &   
 \includegraphics[trim= 0 0 0 0, clip,width=0.33\textwidth]{imgs/kernels_masks/first_round/dinner.jpg} \\
    \end{tabular}
    \caption{Caption}
    \label{fig:kernels_grid_Lai}
\end{figure}

\begin{figure}
    \centering
    \begin{tabular}{*{3}{c}} 
    (a) & (b) & (c) \\
    \includegraphics[trim= 0 0 0 0, clip,width=0.33\textwidth]{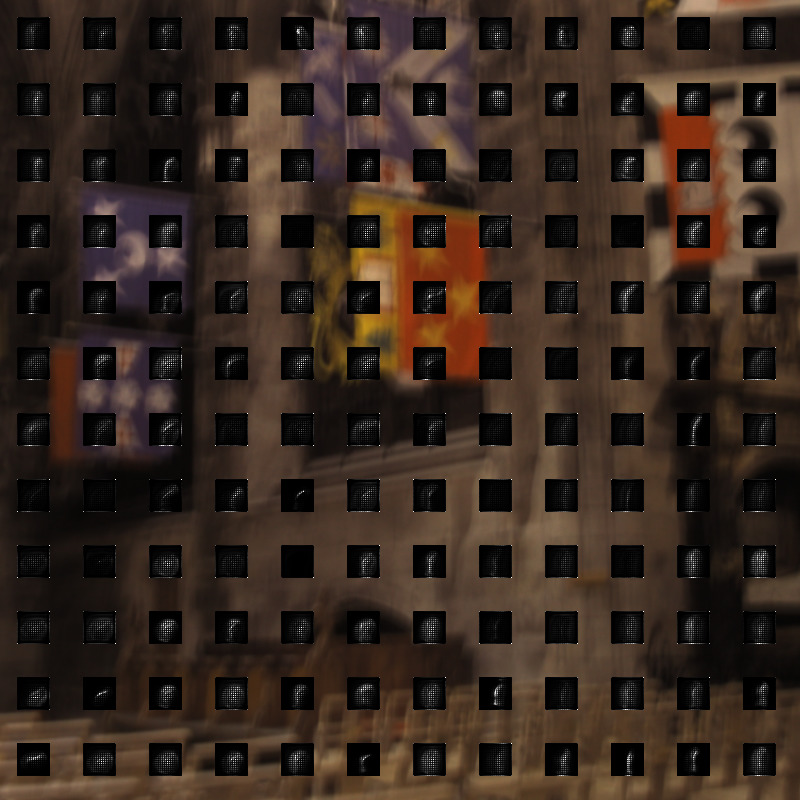} &
    \includegraphics[trim= 0 0 0 0, clip,width=0.33\textwidth]{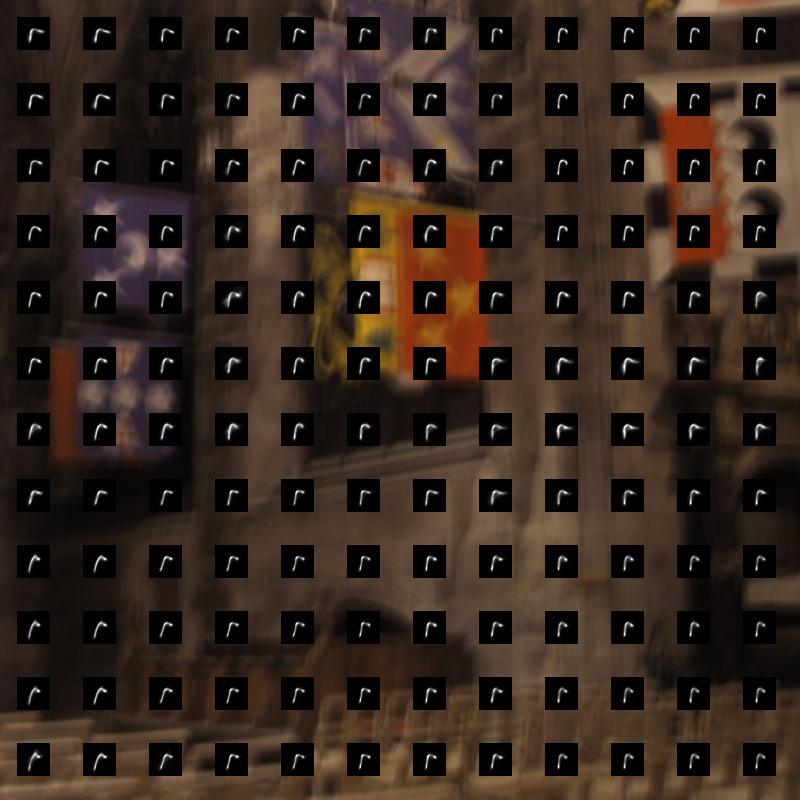}  &   
 \includegraphics[trim= 0 0 0 0, clip,width=0.33\textwidth]{imgs/kernels_masks_NoFC_GoPro_only_reblur_gc/Blurry1_6.jpg}   \\
 \includegraphics[trim= 0 0 0 0, clip,width=0.33\textwidth]{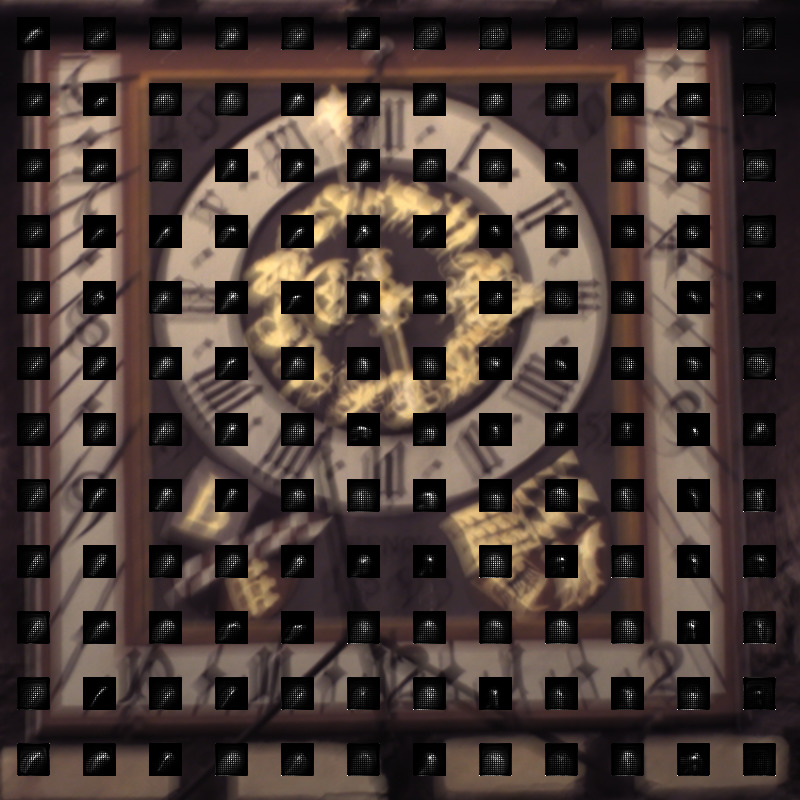} &
    \includegraphics[trim= 0 0 0 0, clip,width=0.33\textwidth]{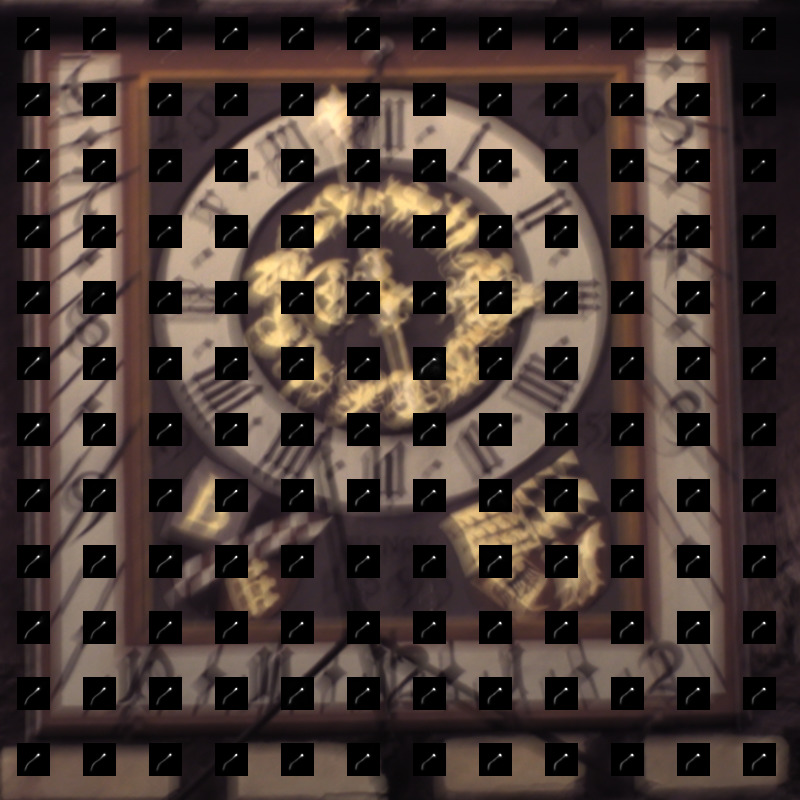}  &   
 \includegraphics[trim= 0 0 0 0, clip,width=0.33\textwidth]{imgs/kernels_masks/first_round/Blurry2_1.jpg} \\
    \end{tabular}
    \caption{Caption}
    \label{fig:kernels_grid_Kohler}
\end{figure}

\subsection{Training using only a reblur loss}

From \cref{tab:reblur_performance_NoFC} it is evident that adding the kernel loss significantly reduce the \textit{reblurring} performance on the GoPro dataset.  In addition, using only the \textit{reblur} loss trains faster. We explored the possibility of obtaining better kernels by constraining the kernel's basis and mixing coefficients predicted by the Kernel Prediction Network. L2 and Total Variation (TV) regularization was evaluated in the final kernels and also TV regularization in the base masks. Table \ref{tab:Xia_gopro_dataset_psnr_reblur} shows the reblur PSNR obtained with and without regularization and Figures  \ref{fig:kernels_grid_035_regs}  and \ref{fig:kernels_grid_276_regs} show some examples. Visually, regularized kernels are preferred, but reblur PSNR is significantly lower. Although regularizing the kernels and mask is an interesting approach to explore, we obtained a better generalization performance when adding the \textit{kernel loss} during training. Also, we found the regularized results very sensitive to the regularization parameters. It is very easy to over-regularize the solution, considerably limiting the expressivity of the Kernel Prediction Network. 

\begin{table}[ht]
    \centering
    \begin{tabular}{l|c}
         Model &         PSNR reblur   \\
         \hline
         No regularization &  40.92 \\
         Masks regularization (TV 1e-9 ) & 40.83 \\
         Masks (TV 1e-9) and kernels (L2 0.1) regularization & 40.96 \\
         Kernels regularization (L2 0.1) &  40.83 \\
         Masks regularization (TV 1e-7 ) & 39.21  \\
         Masks (TV 1e-7) and kernels (L2 1) regularization  &  37.54 \\ 
         \hline
    \end{tabular}
    \caption{Models trained from scratch for 750 epochs.}
    \label{tab:Xia_gopro_dataset_psnr_reblur}
\end{table}

\begin{figure}
     \centering
    \begin{subfigure}[t]{0.3\textwidth}
         \includegraphics[width=\textwidth]{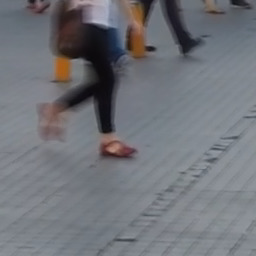}
         \subcaption{Blurry image }
     \end{subfigure}
     \hfill
    \begin{subfigure}[t]{0.3\textwidth}
         \includegraphics[width=\textwidth]{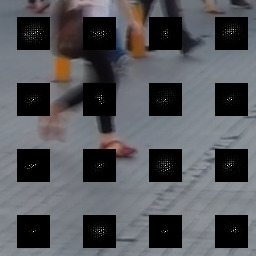}
         \subcaption{No regularization. PSNR~reblur~=~42.61. }
     \end{subfigure}
     \hfill
     \begin{subfigure}[t]{0.3\textwidth}
         \includegraphics[width=\textwidth]{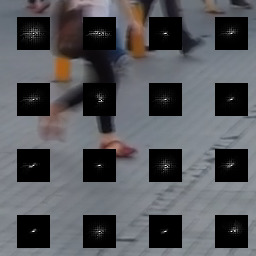}
         \subcaption{Kernels regularization (L2 0.1). PSNR~reblur~=~43.21. }
     \end{subfigure}    
    \begin{subfigure}[t]{0.3\textwidth}
         \includegraphics[width=\textwidth]{imgs/kernels_grid/kernels_reg_01_masks_reg_1e-9/035/loss_0.0000478_psnr_43.21_img_399_kernel_grid_estimated.jpg}
         \subcaption{Kernels (L2 0.1) and masks (TV 1e-9). PSNR~reblur~=~43.21.}
     \end{subfigure}
     \hfill
     \begin{subfigure}[t]{0.3\textwidth}
         \includegraphics[width=\textwidth]{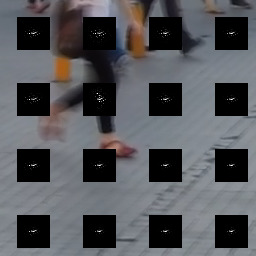}
         \subcaption{Masks (TV 1e-7). PSNR~reblur~=~41.14.}
     \end{subfigure}
      \hfill
     \begin{subfigure}[t]{0.3\textwidth}
         \includegraphics[width=\textwidth]{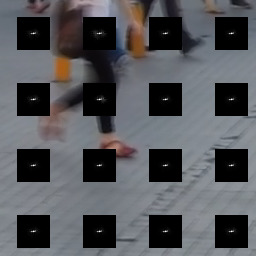}
         \subcaption{Kernels (L2 1) and masks (TV 1e-7). PSNR~reblur~=~39.88.}
     \end{subfigure}
     \caption{Training using only GoPro for \textcolor{red}{ADD} number of epochs.}
     \label{fig:kernels_grid_035_regs}
\end{figure}

\begin{figure}
     \centering
    \begin{subfigure}[t]{0.3\textwidth}
         \includegraphics[width=\textwidth]{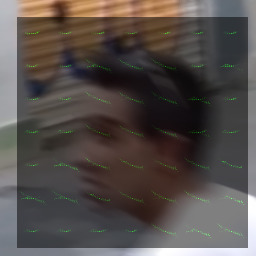}
         \subcaption{Single image overfitting. PSNR~reblur = 45.63 }
     \end{subfigure}
     \hfill
    \begin{subfigure}[t]{0.3\textwidth}
         \includegraphics[width=\textwidth]{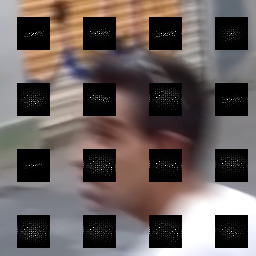}
         \subcaption{No regularization. PSNR~reblur~=~38.89. }
     \end{subfigure}
     \hfill
     \begin{subfigure}[t]{0.3\textwidth}
         \includegraphics[width=\textwidth]{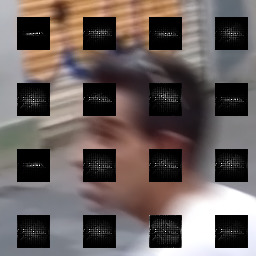}
         \subcaption{Kernels regularization (L2 0.1). PSNR~reblur~=~38.20. }
     \end{subfigure}    
    \begin{subfigure}[t]{0.3\textwidth}
         \includegraphics[width=\textwidth]{imgs/kernels_grid/kernels_reg_01_masks_reg_1e-9/276/loss_0.0001515_psnr_38.20_img_276_kernel_grid_estimated.jpg}
         \subcaption{Kernels (L2 0.1) and masks (TV 1e-9). PSNR~reblur~=~38.20.}
     \end{subfigure}
     \hfill
     \begin{subfigure}[t]{0.3\textwidth}
         \includegraphics[width=\textwidth]{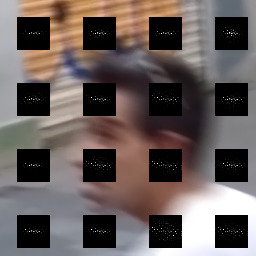}
         \subcaption{Masks (TV 1e-7). PSNR~reblur~=~38.57.}
     \end{subfigure}
      \hfill
     \begin{subfigure}[t]{0.3\textwidth}
         \includegraphics[width=\textwidth]{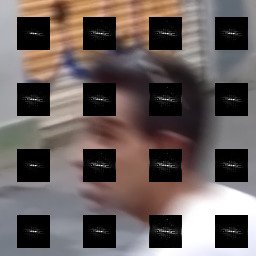}
         \subcaption{Kernels (L2 1) and masks (TV 1e-7). PSNR~reblur~=~35.75.}
     \end{subfigure}
     \caption{TTraining using only GoPro for \textcolor{red}{ADD} number of epochs.}
     \label{fig:kernels_grid_276_regs}
\end{figure}
