# Supplementary material for: Blind Motion Deblurring with Pixel-Wise Kernel Estimation via Kernel Prediction Networks
Source: arXiv:2308.02947 source file (2023-08-05)
Supplement: Supplementary file 6 [file supp_mat_on_losses_effect.tex]

\begin{table}[h]
    \small 
    \caption{\textbf{Cross-dataset evaluation on the RealBlurDataset \cite{rim_2020_ECCV}.} The PSNR/SSIM scores for the classical variational methods (first three rows) were taken from the RealBlur benchmark \cite{rim_2020_ECCV}. For DL-based methods, the values were computed using the models provided by the authors.
    }
    \label{tab:losses_effect_RealBlurDataset}
     \centering
    \begin{tabular}{lcccccc}
    \toprule
    Method & PSNR & SSIM & LPIPS & BS(11)$\uparrow$ & CPBD $\uparrow$ & SI $\uparrow$\\
    \midrule
\textcolor{magenta}{JMKPD (180k)} & 28.68 &  \colorbox{yellow}{0.879} & 0.148 & 0.378 & 0.427 & 3346 \\
\hdashline
\textcolor{magenta}{JMKPD (blurred)} & \colorbox{cyan}{29.04} &  \colorbox{cyan}{0.883}  & 0.146 & 0.399 & 0.336 & 2219  \\
    \bottomrule
    \end{tabular}
\end{table}
